# Supplementary material for: Topological-to-Topological Transition Induced by On-Site Nonlinearity in a One-Dimensional Topological Insulator
Source: arXiv:2501.10087 source file (2025-01-17)

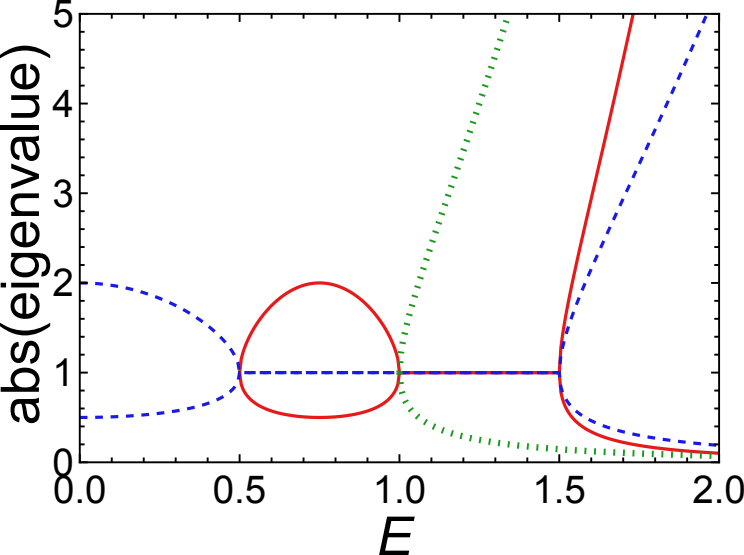

Supplement: Supplementary file 2 [file supplefig_linear_stability.pdf]
